# Supplementary material for: Automated Repair of Neural Networks
Source: arXiv:2207.08157 source file (2022-07-17)
Supplement: Supplementary file 1 [file appendix2.tex]

\section{Quantifier Elimination and Cylindrical Algebraic Decomposition}
\label{appendix:qecad}

%\section{Quantifier Elimination and Cylindrical Algebraic Decomposition}\label{appendix:qecad}

In the following we shall define the task of quantifier elimination (QE). Then, we describe Cylindrical Algebraic Decomposition (CAD), and how it is used to solve QE, or SMT formulas under the NRA theory (as implemented in Z3 \cite{de2008z3}). \textbf{Acknowledgement}: This summary, including its figures, is based on a recent comprehensive CAD tutorial provided in \cite{cadtut18}.

\subsection{QE}

\subsubsection*{Tarski formula} \cite{tarski1951decision} is a formula made of polynomial equations or inequalities, linked by boolean operators ($\lor, \land, \lnot$), for example: $x^2 > 0 \land x^3 - 1 = 0$. The formula may also contain existential or universal quantifiers over the variables forming these equations. The quantification statements may relate to all variables (fully quantified) or some of them (partially quantified). For instance consider the following partially quantified formula: 

\[ \forall{x} \; . x^2 + bx + 1 > 0 \]

In this case, the equivalent quantifier-free formula will depend only on $b$. Throughout this summary, that will be our formula of study.

\begin{definition}[Quantifier elimination] Quantifier elimination is the problem of finding logically equivalent quantifier free formula, where the input is a (partially or fully quantified) Tarski formula. 
\end{definition}

QE can also be the problem of removing a particular number of quantifiers, i.e., not necessarily all of them. Note that the result of QE could be an absolute truth value, under the condition that all variables are quantified (e.g., consider the formula: $\exists{x} \; . x^2 + 1 < 0$). Additionally, the order of quantification matters and may lead to different results.

\subsection{CAD}

\subsubsection*{Semi-Algebraic Set} is a subset of $\mathbb{R}^n$ defined by either: 
\begin{enumerate}
	\item Finite conjunction of polynomial equations (and/or inequalities) in $n$ variables; or,
	\item The finite union of such sets
\end{enumerate}

For example: $\phi = x^2 + y^2 -1 > 0 \land y - x > 0 \land x > 0$ satisfies (1)  and defines the set which correspond to the blue region in Figure \ref{fig:semialg}. 

Every Tarski logic formula defines a geometric semi-algebraic set.

\begin{figure}
	\centering
	\includegraphics[scale=0.25]{graphics/semi_alg_set.png}
	\caption{The semi algebraic set as defined by $\phi$}
	\label{fig:semialg}
\end{figure}

\subsubsection*{A decomposition} of $\mathbb{R}^n$ is a conjunction of cells $D_i$ such that: 
\begin{itemize}
    \item $D_i \cap D_j = \emptyset$, and
    \item $\bigcup\limits_{i} D_{i} = \mathbb{R}^n$
\end{itemize}

We want to build \textit{decomposition} where the sets are \textit{semi-algebraic}. Our desire is that the decomposition will be \textbf{truth-invariant} for the quantifier free part of \textit{Tarski} formula being studied - i.e. within any given cell, the formula is either true or false throughout. Then, each cell can be tagged with a truth label, which enables solving QE. Algorithms used to build such decompositions also impose these two additional constraints:

\begin{enumerate}
	\item Each cell is \textbf{Cylindrical} - i.e. it may be described by conditions: $c_1(x_1)$, $c_2(x_1, x_2)$ ,..., $c_n(x_1,..., x_n)$, where each $c_i$ is one of:
	\begin{itemize}
		\item $l_i(x_1,..., x_{i-1}) < x_i $
		\item $l_i(x_1,..., x_{i-1}) < x_i < u_i(x_1,..., x_{i-1})$
		\item $x_i < u_i(x_1,..., x_{i-1})$
		\item $x_i = s_i(x_1,..., x_{i-1})$
	\end{itemize}
		and $l_i,u_i,s_i$ are functions in $i-1$ variables. An example for such cells can be seen in Figure \ref{fig:cylcells}\\
		
	\item A composition is \textbf{Cylindrically Arranged} if for any two cells $D_i, D_j$ ($i \neq j$), the projections onto $\mathbb{R}^k$, for all $k < n$, are equal or disjoint, where $n$ denotes the number of variables in the formula. For example the following cylindrical cells are cylindrically arranged: $D_i = \{ y < f(x) , -1 < x < 1 \}$ and $D_j = \{ 0 < y < g(x), -1 < x < 1 \}$. An example for non cylindrically arranged cells can be seen at Figure \ref{fig:cylarranged}.
\end{enumerate}

\textbf{Crucial point:} Both conditions are made w.r.t variable ordering. 

\begin{figure}
	\centering
	\includegraphics[scale=0.125]{graphics/cylindrical_cell}
	\caption{A union of cylindrical cells.}
	\label{fig:cylcells}
\end{figure}

\begin{figure}
	\centering
	\includegraphics[scale=0.15]{graphics/non_cyl_arranged.png}
	\caption{Two cells which are not cylindrically arranged. Observe their projections onto the $x$ axis, they are neither equal or disjoint since they overlap.}
	\label{fig:cylarranged}
\end{figure}

\begin{definition}[CAD] CAD is a decomposition of $\mathbb{R}^n$ into semi-algebraic cylindrical cells, that are cylndrically arranged. \cite{collins1975quantifier}
\end{definition}

Recall that we want a CAD \textbf{truth-invariant} for our formula of study, while Collins algorithm \cite{collins1975quantifier} provides CAD that is \textbf{sign-invariant} - i.e. each polynomial has a constant sign (positive, negative, zero) in each cell. A CAD \textbf{sign-invariant} for the polynomials in the formula, is also \textbf{truth-invariant}, however will be likely harder to compute.

\subsubsection*{Example: Circle Semi-Algebraic}

A CAD of $\mathbb{R}^2$ sign-invariant for $x^2 + y^2 -1$ must have 13 cells. Assuming we project onto the $x-axis$, then the semialgebraic cells are as follows:

\begin{equation*}
	\begin{aligned}
		x < -1 : & \{ [x < -1, y = y] \} \\
		x = -1 : & \{ [x = -1, y < 0], [x = -1, y = 0], [x = -1, y > 0] \} \\
		-1 < x < 1 : & \{ [-1 < x < 1, y^2 + x^2 - 1 > 0, y < 0], [-1 < x < 1, y^2 + x^2 - 1 = 0, y < 0],  \\
		             & [-1 < x < 1, y^2 + x^2 - 1 < 0], [-1 < x < 1, y^2 + x^2 - 1 = 0, y > 0], \\
		             & [-1 < x < 1, y^2 + x^2 - 1 < 0, y > 0] \} \\
		x = 1 : & \{ [x = 1, y < 0], [x = 1, y = 0], [x = 1, y > 0] \} \\
		x > 1 : & \{ [x > 1, y = y] \} \\
	\end{aligned}
\end{equation*}

Depicted in Figure \ref{fig:cell_decomp_vis} is the decomposition visualization of the first 3 cells.

\begin{figure}[!htb]
	\minipage{0.32\textwidth}
	\includegraphics[width=\linewidth]{graphics/decomp_vis_cell1.png}
	%\caption{A really Awesome Image}\label{fig:awesome_image1}
	\endminipage\hfill
	\minipage{0.32\textwidth}
	\includegraphics[width=\linewidth]{graphics/decomp_vis_cell2.png}
	%\caption{A really Awesome Image}\label{fig:awesome_image2}
	\endminipage\hfill
	\minipage{0.32\textwidth}%
	\includegraphics[width=\linewidth]{graphics/decomp_vis_cell3.png}
	
	\endminipage
	\caption{The most left figure depicts the first cell: $\{x < -1, y \; free\}$. Middle figure represents the second cell: $\{x = -1, y < 0\}$, while the rightmost figure depicts the third cell: $\{x = -1, y = 0\}$.  }\label{fig:cell_decomp_vis}
\end{figure}

The cylindricity means we can think of CAD as a tree branching by cylindrical cell variable restriction, as can be seen in Figure \ref{fig:cad_tree}.

\begin{figure}
	\centering
	\includegraphics[scale=0.3]{graphics/cad_tree.png}
	\caption{CAD as a tree branching by cylinrical cell variable restriction.}
	\label{fig:cad_tree}
\end{figure}

\subsection*{Traditional CAD algorithm}
Collins algorithm for CAD first projects a problem from $\mathbb{R}^n$ down to a real line in $\mathbb{R}^1$; and then it incrementally builds CAD by dimension. This process can be described by two steps:

\begin{enumerate}
	\item \textbf{Projection}: Identifies polynomials with lower dimensions necessary to build the CAD.
	\item \textbf{Lifting}: Uses these polynomials to construct the cells.
\end{enumerate}

\subsection*{Projection}

\subsubsection*{Projection operator} $P$ takes polynomials in $k$ variables, and produces another set in $k-1$ variables. (the operator identifies polynomials which describe important changes in behavior: discriminatns, coefficients, etc.). Additionally, we project under variable ordering.

\subsubsection*{Projection example} $P(x^2 + y^2 + z^2 -1) = x^2 + y^2 -1$, and then $P(x^2 + y^2 -1) = (x-1)(x+1)$.

\subsection*{Lifting}

CAD of $\mathbb{R}^n$ is constructed incrementally as follows:

\begin{itemize}
	\item \textbf{Base case}: A CAD of $\mathbb{R}$ is produced using the roots of the univariate polynomials, and the intervals in between.
	\item \textbf{Generic case}: Suppose we have a CAD of $\mathbb{R}^k$, to construct a CAD of $\mathbb{R}^{k+1}$, do the following for each cell in $\mathbb{R}^k$:
\end{itemize}

\begin{enumerate}
	\item Consider the cylinder over the cell (e.g., suppose we have a CAD of $\mathbb{R}$, and cell $D$ which is an interval of $\mathbb{R}$. Then the cylinder over $D$ is $D \times \mathbb{R}$)
	\item Identify the projection polynomials with main variable $X_{k+1}$ and evaluate each at a \textbf{sample point} of the cell.
	\item Find the roots of these univariate polynomials.
	\item Construct a stack over the cell: a collection of cells of $\mathbb{R}^{k+1}$. These consist of \textit{sections} (where polynomial has a root) and \textit{sectors} (the intervals in-between).
\end{enumerate}

Together, the stacks form a CAD of $\mathbb{R}^{k+1}$.

\subsubsection*{Example: Circle Semi-Algebraic}

Consider again the circle $f = x^2 + y^2 -1$, then $P(f) = \{x-1, x+1\}$. The roots are $x=1, x=-1$, so a CAD of $\mathbb{R}^{1}$ is produced with 5 cells. \\

Consider the cell where $-1 < x < 1$, we can take the sample point $x=0$ which leads to $f_{x=0} = y^2 -1 $. $f_{x=0}$ has two roots, thus, the stack over the cell consists of two \textbf{sections} and three \textbf{sectors}. \\

Combining the stacks for cells in $\mathbb{R}^{1}$ gives the CAD of $\mathbb{R}^{2}$ with 13 cells.

\subsection*{Example: QE with CAD}

We go back to our formula of study: $\forall{x} \; . x^2 + bx + 1 > 0 \equiv (\exists x \; . x^2 + bx + 1 <= 0)$. In the following we describe the steps required to build a sign-invariant CAD for $\exists x \; . x^2 + bx + 1 <= 0$ and eliminate the quantifier in this formula.

\subsubsection*{Projection} Applying projection results in: $P(f) = \{ b^2 - 4\}$, and we have real roots at $b=2, b=-2$. As a result, 5-cell CAD of $\mathbb{R}^{1}$ is built.

\subsubsection*{Lifting} Pick a \textit{sample point} for $b$ in each cell. For the first cell we let $b=-5/2$, hence $f_{b=-5/2}= \frac{1}{2} (2x - 1)(x - 2)$. We infer 5-cell stack (2 sectors, and 3 sections). Then, we pick sample points for the sectors.

We repeat this process to build stacks over the other 4 cells in $\mathbb{R}^{1}$, to obtain a 17-cell CAD of $\mathbb{R}^{2}$ (2 points, 8 line segments, 7 plane segments). We then tag each with a truth value for $x^2 + bx + 1 <= 0$ (8 True, 9 False) via sample point test. 

Finally, for solving $\exists x \; . x^2 + bx + 1 <= 0$, we project the true cells of $\mathbb{R}^{1}$: $ \{b < -2, b = 2, b = 2, b > 2 \}$. Lastly, we take the complement of these cells (other cells in $\mathbb{R}^{1}$) and find $-2 < b < 2$. This inference step can also be seen in Figure \ref{fig:qe_cad}.

\begin{figure}
	\centering
	\includegraphics[scale=0.2]{graphics/qe_cad.png}
	\caption{Quantifier elimination applied on $\exists x \; . x^2 + bx + 1 <= 0$, by projecting the true cells of $\mathbb{R}^{1}$, and inferring the complement cell which is the interval $-2 < b < 2$. Red and green dots depict the sample points, green correspond to true cells, while red refers to false cells.}
	\label{fig:qe_cad}
\end{figure}

\subsection*{CAD complexity}
If the input has $m$ polynomials in $n$ variables of degree at most $d$ in any one variable, then the complexity is in the order: $2dm^{2^{O(n)}}$

\subsection*{NLSAT}
The NLSAT algorithm \cite{de2008z3} that we employ in our framework does not build CAD but uses CAD technology. The algorithm follows the SMT strategy of iteratively forming model and learning from conflicts. When a conflict occurs, it learns the cylindrical cell where it occurs via projection and lifting, \textbf{only for that cell}.
